# Supplementary material for: Trade-Offs Between Ranking Objectives: Descriptive Evidence and Structural Estimation
Source: arXiv:2210.16408 source file (2026-03-25)
Supplement: Supplementary file 2 [file appendix_table_summary_stats_er.tex]

\begin{table}[tb] \centering \footnotesize
\caption{Summary statistics (Expedia ranking)} \label{tab:summary_stats_er}

\begin{threeparttable}
\begin{tabular}{lllccccc} 
\midrule

 && \multicolumn{1}{c}{N} & \multicolumn{1}{c}{Mean} & \multicolumn{1}{c}{Median} & \multicolumn{1}{c}{Std. Dev} & \multicolumn{1}{c}{Min.} & \multicolumn{1}{c}{Max.} \\
\midrule
\bfseries{Hotel-level} \\
\hspace{1em}\hspace{1em}Price (in \$)&&3,146,022&154.54&129.00&96.54&10.00&1000.00\\
\hspace{1em}\hspace{1em}Star rating&&3,084,716&\hphantom{00}3.31&\hphantom{00}3&\hphantom{0}0.87&\hphantom{0}1&\hphantom{0}5\\
\hspace{1em}\hspace{1em}Review score&&3,143,741&\hphantom{00}3.92&\hphantom{00}4.00&\hphantom{0}0.80&\hphantom{0}0.00&\hphantom{0}5.00\\
\hspace{1em}\hspace{1em}No reviews&&3,143,741&\hphantom{00}0.02&\hphantom{00}0&\hphantom{0}0.13&\hphantom{0}0&\hphantom{0}1\\
\hspace{1em}\hspace{1em}Chain&&3,146,022&\hphantom{00}0.68&\hphantom{00}1.00&\hphantom{0}0.47&\hphantom{0}0.00&\hphantom{0}1.00\\
\hspace{1em}\hspace{1em}Location score&&3,146,022&\hphantom{00}3.13&\hphantom{00}3&\hphantom{0}1.50&\hphantom{0}0&\hphantom{0}7\\
\hspace{1em}\hspace{1em}On promotion&&3,146,022&\hphantom{00}0.26&\hphantom{00}0&\hphantom{0}0.44&\hphantom{0}0&\hphantom{0}1\\
\midrule
\bfseries{Session-level} \\
\hspace{1em}\hspace{1em}Number of items&&114,529&\hphantom{0}27.47&\hphantom{0}31&\hphantom{0}7.91&\hphantom{0}5&\hphantom{00}38\\
\hspace{1em}\hspace{1em}Number of clicks&&114,529&\hphantom{00}1.11&\hphantom{00}1&\hphantom{0}0.59&\hphantom{0}1&\hphantom{00}24\\
\hspace{1em}\hspace{1em}Made booking&&114,529&\hphantom{00}0.92&\hphantom{00}1&\hphantom{0}0.28&\hphantom{0}0&\hphantom{0}1\\
\hspace{1em}\hspace{1em}Trip length (in days)&&114,529&\hphantom{00}2.13&\hphantom{00}2&\hphantom{0}1.67&\hphantom{0}1&\hphantom{00}38\\
\hspace{1em}\hspace{1em}Booking window (in days)&&114,529&\hphantom{0}32.78&\hphantom{0}14&48.16&\hphantom{0}0&\hphantom{0}482\\
\hspace{1em}\hspace{1em}Number of adults&&114,529&\hphantom{00}1.96&\hphantom{00}2&\hphantom{0}0.87&\hphantom{0}1&\hphantom{0}9\\
\hspace{1em}\hspace{1em}Number of children&&114,529&\hphantom{00}0.37&\hphantom{00}0&\hphantom{0}0.77&\hphantom{0}0&\hphantom{0}9\\
\hspace{1em}\hspace{1em}Number of rooms&&114,529&\hphantom{00}1.11&\hphantom{00}1&\hphantom{0}0.42&\hphantom{0}1&\hphantom{0}8\\
\midrule 
\end{tabular}
\begin{tablenotes}
\item \footnotesize{\emph{Notes:} Summary statistics as in Table \ref{tab:summary_stats_rr} for sessions 
   under Expedia ranking. }
\end{tablenotes} 
\end{threeparttable}
\end{table}
